# Supplementary material for: OxfordTVG-HIC: Can Machine Make Humorous Captions from Images?
Source: arXiv:2307.11636 source file (2023-07-21)
Supplement: Supplementary file 1 [file figrue_new_teaser.tex]

\begin{figure}[h]
\resizebox{\columnwidth}{!}{%
\includegraphics[width=\linewidth]{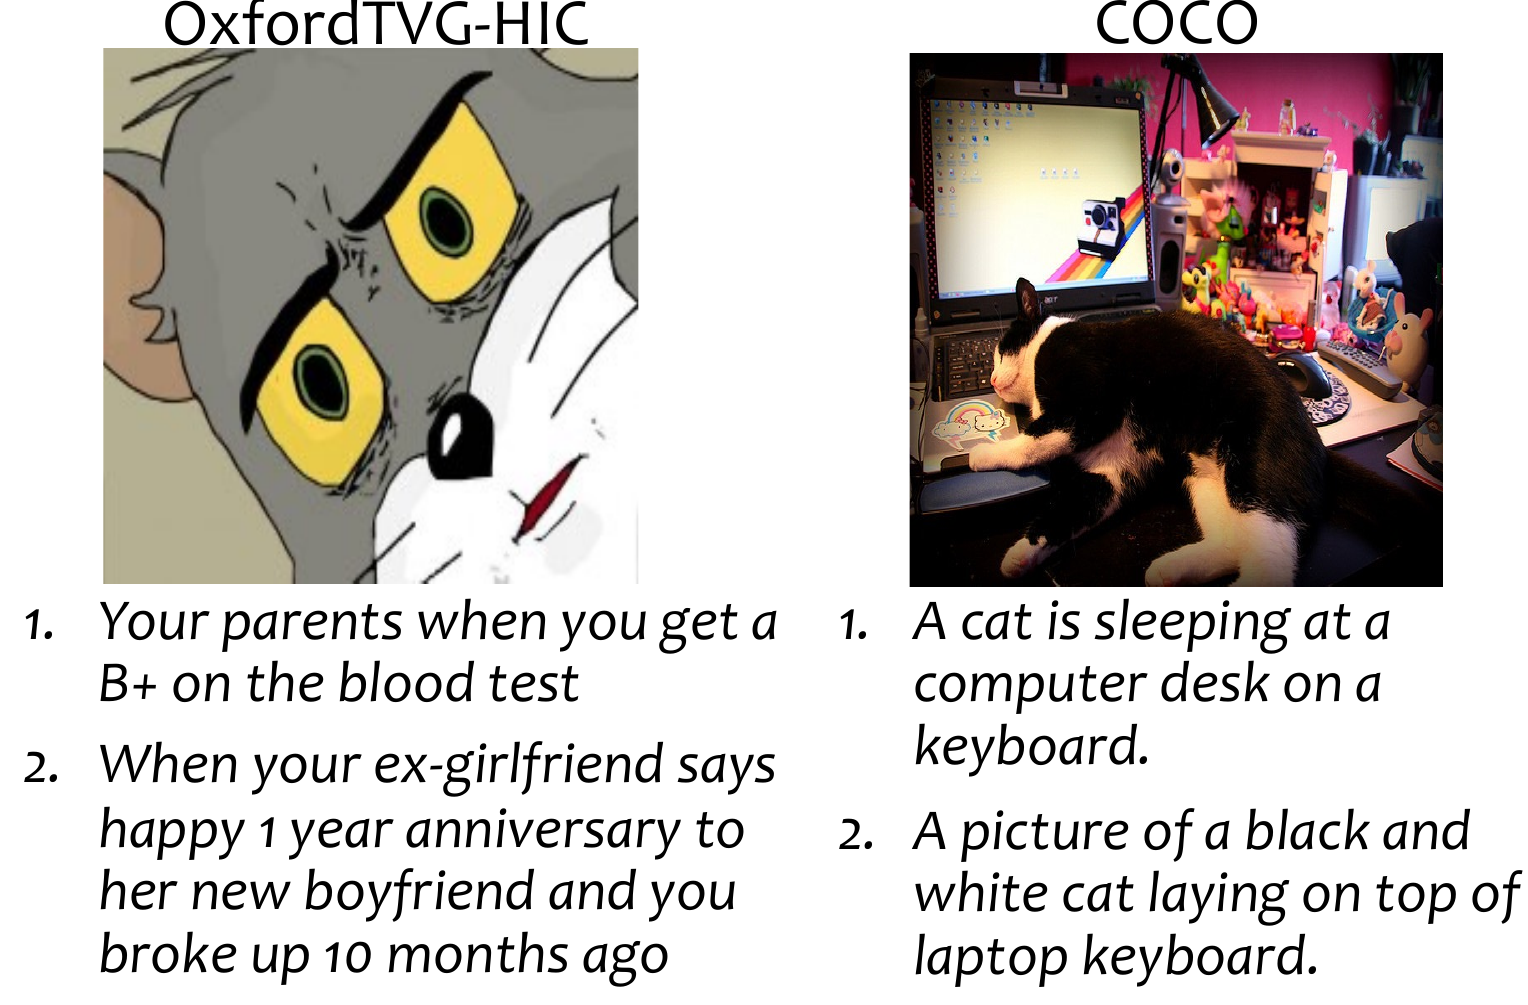}
\centering
}
\caption{Corrected image-text sample comparison from \dname~and COCO~\cite{mscoco}
}
\label{fig:correct_dataset_teaser}
\end{figure}
