# Supplementary material for: OxfordTVG-HIC: Can Machine Make Humorous Captions from Images?
Source: arXiv:2307.11636 source file (2023-07-21)
Supplement: Supplementary file 2 [file figure_new_data_semantics.tex]

\begin{figure}[h]
\resizebox{\columnwidth}{!}{%
\includegraphics[width=\linewidth]{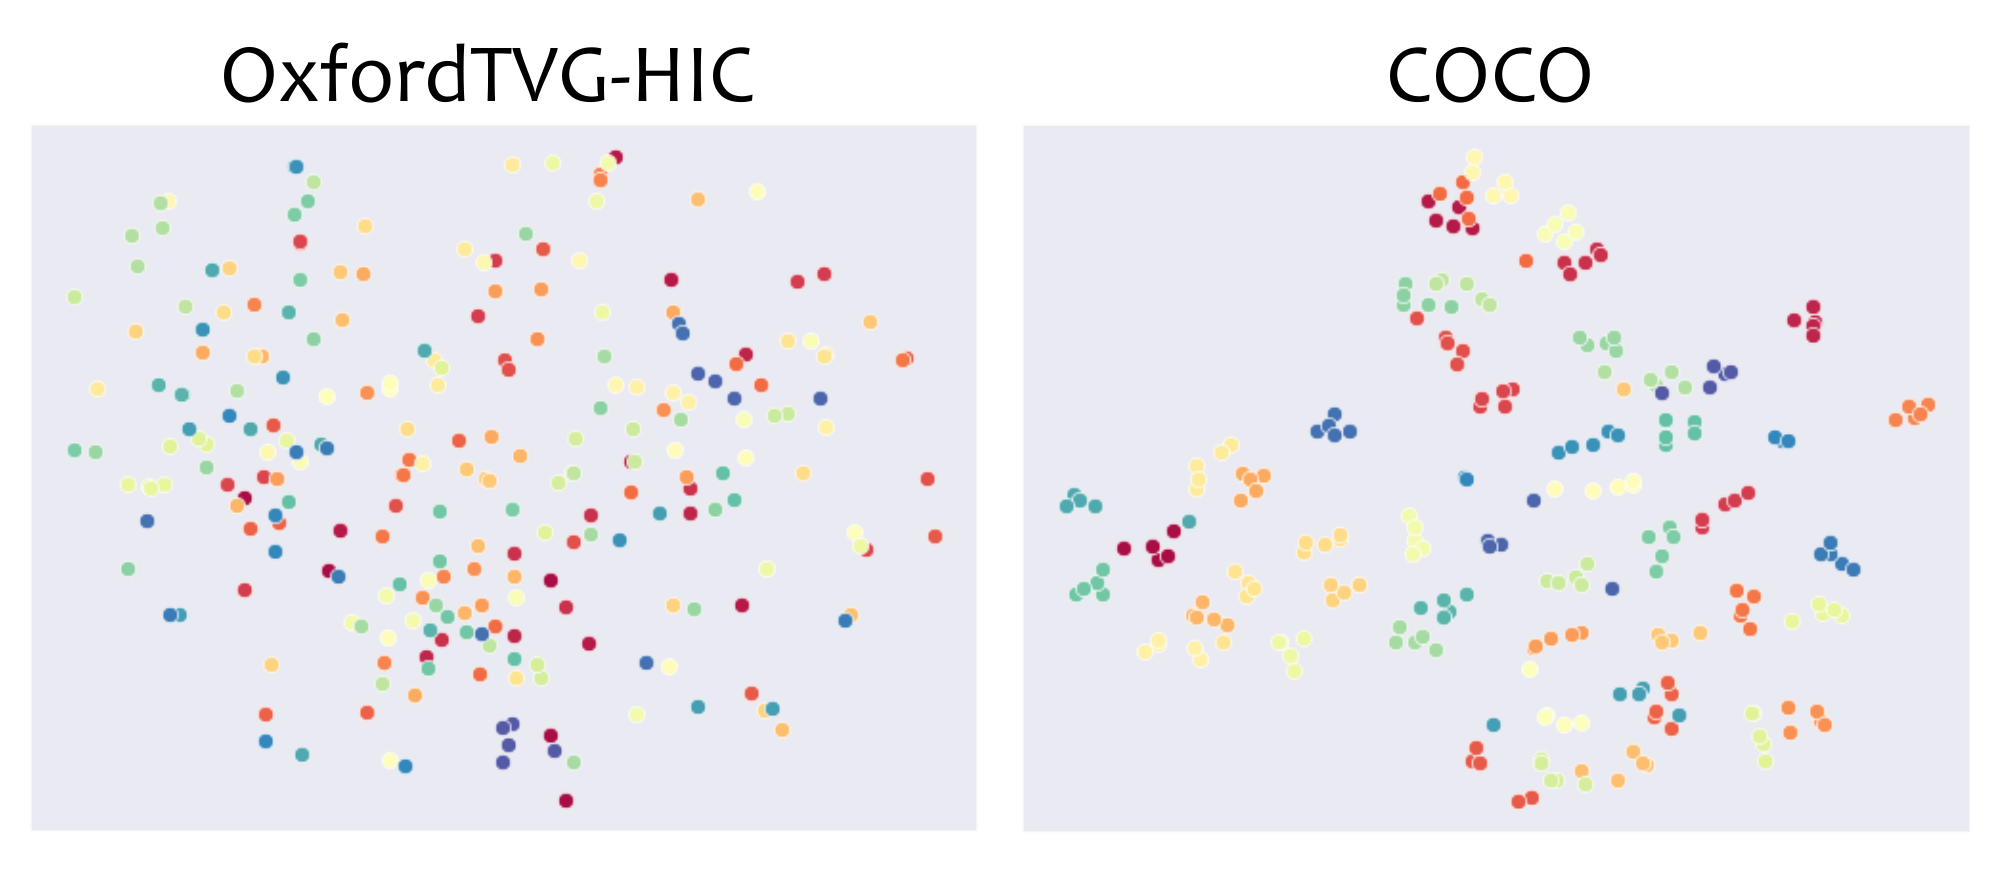}
\centering
}
\caption{Corrected caption semantic embedding distribution from \dname~and COCO~\cite{mscoco}
}
\label{fig:correct_dataset_semantics}
\end{figure}
