# Supplementary material for: OxfordTVG-HIC: Can Machine Make Humorous Captions from Images?
Source: arXiv:2307.11636 source file (2023-07-21)
Supplement: Supplementary file 3 [file figure_new_data_stats.tex]

\begin{figure}[h]
\resizebox{\columnwidth}{!}{%
\includegraphics[width=\linewidth]{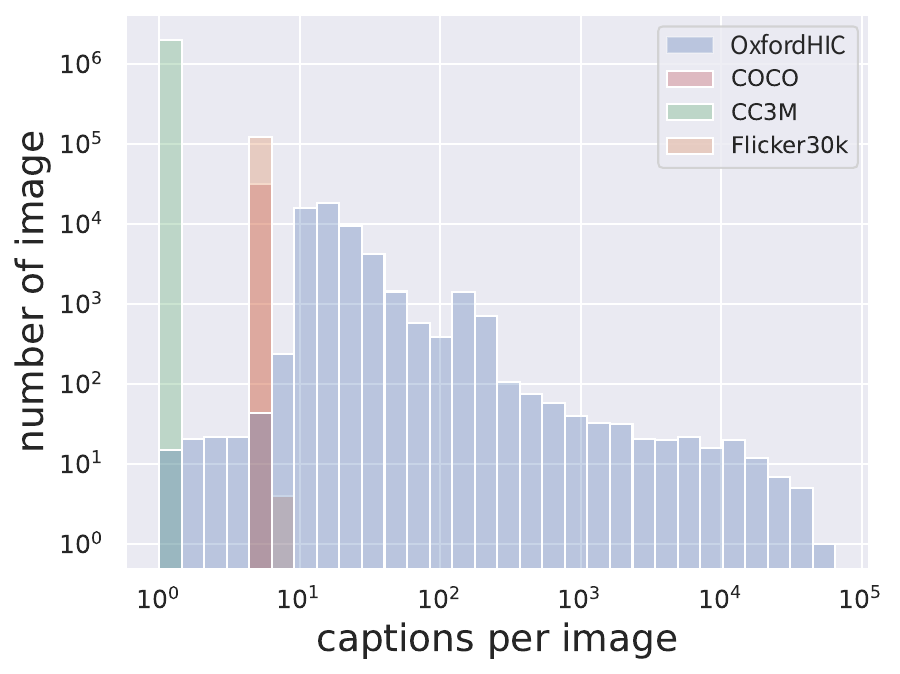}
\centering
}
\caption{Corrected number of captions per image distribution histogram for \dname~and object-centric datasets~\cite{mscoco, conceptual, flicker} 
}
\label{fig:correct_dataset_statistics}
\end{figure}
